# Supplementary material for: Science cases for a visible interferometer
Source: arXiv:1703.02395 source file (2017-03-21)
Supplement: Supplementary file 1 [file appendix.tex]

\begin{appendix}
\chapter{Appendix}

\section{Appendices}\label{appendix}\index{appendix}
Appendices should be used only when absolutely necessary. They
should come before the References. If there is more than one
appendix, number them alphabetically. Number displayed equations
occurring in the Appendix in this way, e.g.~(\ref{appeq1}), (A.2),
etc.

\begin{equation} \mu(n, t) = \frac{\sum^\infty_{i=1} 1(d_i < t,
N(d_i) = n)} {\int^t_{\sigma=0} 1(N(\sigma) = n)d\sigma}\,.
\label{appeq1}
\end{equation}

Sectional units are obtained in the usual way, i.e. with the
\LaTeX{} instructions \verb|\section|, \verb|\subsection|.

\begin{table}[h]
\tbl{Class options.$^{\textrm a}$}{
\begin{tabular}{@{}lll@{}}
\toprule
Option & \multicolumn{2}{c}{Purpose} \\\colrule
& Even page headers& Odd page headers\\[3pt]\cline{2-3}\\[-4pt]
{\tt acrhead}& Author Name(s) & Chapter Title\\
{\tt csrhead}& Chapter Title & Section Title\\
{\tt bcrhead} default & Book Title & Chapter Title\\[12pt]
\begin{minipage}{.6in}{{\tt onethmnum}}\vspace*{51pt}\ \end{minipage} & \multicolumn{2}{l}{\begin{minipage}{2.3in}{To number all theorem-like objects in a
single sequence, e.g. Theorem~1, Definition 2,\\ Lemma 3, etc.\\
Default: individual numbering on different\\ theorem-like objects, e.g. Theorem 1,\\ Definition 1, Lemma 1, etc.}
\end{minipage}}\\
\\[-1pt]
{\tt wsdraft} & \multicolumn{2}{l}{To draw border line around text area.}\\[6pt]
{\tt bigtoc}  & \multicolumn{2}{l}{To align the table of contents}\\
              & \multicolumn{2}{l}{for those books with more than 9 Chapters}\\
\botrule
\end{tabular}}
\begin{tabnote}
$^{\textrm a}$Usage: \verb|\documentclass[option]{ws-book975x65}|
\end{tabnote}
\end{table}

\subsection{Appendix sectional units}
Sample text.
\begin{tablehere}
\tbl{Commonly used macros.}{
\begin{tabular}{@{}ll@{}}
\toprule
Macro/Environment name&Purpose\\
\colrule
{\tt$\backslash$chapter[\#1]}\{{\tt\#2}\} & Chapter title\\
{\tt$\backslash$section}\{{\tt\#1}\} & Section heading\\
{\tt$\backslash$subsection}\{{\tt\#1}\} & Subsection heading\\
{\tt$\backslash$subsubsection}\{{\tt\#1}\} & Subsubsection heading\\
{\tt$\backslash$section*}\{{\tt\#1}\} & Unnumbered Section head\\
{\tt$\backslash$begin}\{{\tt{itemlist}}\} & Start bulleted lists\\
{\tt$\backslash$end}\{{\tt{itemlist}}\} & End bulleted lists\\
{\tt$\backslash$begin}\{{\tt{arabiclist}}\} & Start arabic lists (1, 2, 3...)\\
{\tt$\backslash$end}\{{\tt{arabiclist}}\} & End arabic lists\\
{\tt$\backslash$begin}\{{\tt{romanlist}}\} & Start roman lists (i, ii, iii...)\\
{\tt$\backslash$end}\{{\tt{romanlist}}\} & End roman lists\\
{\tt$\backslash$begin}\{{\tt{Romanlist}}\} & Start roman lists (I, II, III...)\\
{\tt$\backslash$end}\{{\tt{Romanlist}}\} & End roman lists\\
{\tt$\backslash$begin}\{{\tt{alphlist}}\} & Start alpha lists (a, b, c...)\\
{\tt$\backslash$end}\{{\tt{alphlist}}\} & End alpha lists\\
{\tt$\backslash$begin}\{{\tt{Alphlist}}\} & Start alpha lists (A, B, C...)\\
{\tt$\backslash$end}\{{\tt{Alphlist}}\} & End alpha lists\\
{\tt$\backslash$begin}\{{\tt{proof}}\} & Start of Proof\\
{\tt$\backslash$end}\{{\tt{proof}}\} & End of Proof\\
{\tt$\backslash$begin}\{{\tt{theorem}}\} & Start of Theorem\\
{\tt$\backslash$end}\{{\tt{theorem}}\} & End of Theorem (see Page \pageref{theo} for detailed list)\\
{\tt$\backslash$begin}\{{\tt{appendix}}\} & Start Appendix\\
{\tt$\backslash$end}\{{\tt{appendix}}\} & End Appendix\\
{\tt$\backslash$begin}\{{\tt{thebibliography}}\}\{{\tt\#1}\} & Start of reference list\\
{\tt$\backslash$end}\{{\tt{thebibliography}}\} & End of reference list\\
{\tt$\backslash$bibitem}[\{{\tt\#1}\}]\{{\tt\#2}\}& reference item in author-date style\\
{\tt$\backslash$bibitem}\{{\tt\#1}\} & reference item in numbered style\\
{\tt$\backslash$bibliographystyle}\{{\tt\#1}\} & To include \btex{} style file\\
{\tt$\backslash$bibliography}\{{\tt\#1}\} & To include \btex{} database\\
{\tt$\backslash$blankpage} & for blank page with no running heads\\[6pt]
\multicolumn{2}{@{}l}{Macros available for Tables/Figures.}\\[3pt]
{\tt figure} & figures\\
{\tt sidewaysfigure} & landscape figures\\
{\tt table} & tables\\
{\tt sidewaystable} & landscape tables\\
{\tt$\backslash$tbl}\{{\tt\#1}\}\{{\tt\#2}\} & \#1 - table caption;\\
& \#2 - tabular environment\\[3pt]
\multicolumn{2}{@{}l}{Horizantal Rules for tables}\\
{\tt$\backslash$toprule} & one rule at the top\\
{\tt$\backslash$colrule} & one rule separating column heads from\\ & data cells\\
{\tt$\backslash$botrule} & one bottom rule\\
{\tt$\backslash$Hline} & one thick rule at the top and bottom of\\ & the tables with multiple column heads\\
\botrule
\end{tabular}}
\end{tablehere}
\enlargethispage{12pt}
\end{appendix}
